# Supplementary material for: RiskBench: A Scenario-based Benchmark for Risk Identification
Source: arXiv:2312.01659 source file (2024-03-05)
Supplement: Supplementary file 1 [file supplementary.tex]

\title{\LARGE \bf
RiskBench: A Scenario-based Benchmark for Risk Identification\\Supplementary Material
}

\author{Chi-Hsi Kung$^{1}$ \, Chieh-Chi Yang$^{1}$ \, Pang-Yuan Pao$^{1}$ \, Shu-Wei Lu$^{1}$ \,  Pin-Lun Chen$^{1}$  \\ Hsin-Cheng Lu$^{2}$ \, Yi-Ting Chen$^{1}$ \\
}

\maketitle
\thispagestyle{empty}
\pagestyle{empty}

%%%%%%%%%%%%%%%%%%%%%%%%%%%%%%%%%%%%%%%%%%%%%%%%%%%%%%%%%%%%%%%%%%%%%%%%%%%%%%%%

\begin{table}[t!]
    \scriptsize
    \centering
    \caption{\textbf{Risk identification results in risk types.} The numbers reported are F1 scores. }      %%%%%% interactive+collision
\begin{tabular}
            {@{}l@{\;} @{\;} @{\;} c @{\;}@{\;}@{\;} @{\;}@{\;}@{\;}c @{\;}@{\;}@{\;} @{\;}@{\;}@{\;} c @{\;}@{\;}@{\;} @{\;}@{\;}@{\;} c @{\;}}
            
            \toprule
             \multirow{1}{*}{ \begin{tabular}{@{\;}c@{\;}} \end{tabular}} & 
             \multicolumn{1}{c}{Four-wheeler }  & 
             \multicolumn{1}{c}{Two-wheeler }  & 
             \multicolumn{1}{c}{Pedestrian}   & 

             \\
             \toprule
             % Kalman Filter~\cite{thrun2002probabilistic}
             %  &  &  &  \\
             % Social-GAN~\cite{social-gan}   
             %  &  & &  \\
             % MANTRA~\cite{mantra}
             %  &  &  & 
             %  \\
             QCNet~\cite{zhou2023query}
             & 57.2 & 61.5 & 14.3
             \\
             
             \midrule
             RRL~\cite{zeng2017agent}
             & 44.5 & 62.6 & 64.3
             \\
             BCP~\cite{li2020make}
             & 44.2 & 21.4 & 29.1 
             \\
             
             \midrule
             RRL+state
             & 59.1 & 62.7 & 69.2
             \\
             BCP+state
             & 55.2 & 34.6 & 42.2
             \\

             \midrule
            \bottomrule
        \end{tabular}
        \label{table:agent_type}

\end{table}

\begin{table*}[t!]
    \scriptsize
    \centering
\caption{\textbf{Temporal Consistency} results calculated within 1, 2, and 3 seconds before the critical/collision point. \hank{we can add a new experiments that tests if filter can help planning-awareness evaluation. A simple way is to use random to disturb the consistency.}}       %%%%%% interactive+obstacle+collision
\begin{tabular}
            {@{}l @{\;}@{\;}@{\;} c @{\;}@{\;}@{\;}  c @{\;}@{\;}@{\;}  c @{\;}@{\;}@{\;}  c @{\;}@{\;}@{\;}  c @{\;}@{\;}@{\;}  c @{\;}@{\;}@{\;} c @{\;}@{\;} @{\;} c @{\;} c @{\;}@{\;}@{\;} c @{\;}@{\;} c @{\;}@{\;}@{\;} c @{\;}@{\;}@{\;}}
            \toprule
            \multirow{2}{*}{ \begin{tabular}{@{\;}c@{\;}} \end{tabular}} & 
             \multicolumn{3}{@{\;}c}{consistency}  & 
             % \multicolumn{1}{@{\;}c}{2s}  & 
             % \multicolumn{1}{@{\;}c}{3s}   & 
             \multicolumn{1}{@{\;}c}{P}   & 
             \multicolumn{1}{@{\;}c}{R}   & 
             \multicolumn{1}{@{\;}c}{F1}   & 
             \multicolumn{1}{@{\;}c}{PIC}   & 
             \multicolumn{2}{@{\;}c@{\;}}{interactive}   & 
             \multicolumn{2}{@{\;}c@{\;}}{obstacle}   & 

             \\
             \cmidrule(lr){2-4}
             \cmidrule(lr){9-10} 
             \cmidrule(lr){11-12}
             &
             \multicolumn{1}{@{\;}c}{1s}&
             \multicolumn{1}{@{\;}c}{2s}&
             \multicolumn{1}{@{\;}c}{3s}& 
              & & & & 
             \begin{tabular}{@{\;}@{\;}c@{\;}}  IR  \end{tabular} & 
             \begin{tabular}{@{\;}c@{\;}}  CR (\%)  \end{tabular} & 
             \begin{tabular}{@{\;}@{\;}c@{\;}}  IR   \end{tabular} & 
             \begin{tabular}{@{\;}c@{\;}}  CR (\%)  \end{tabular} & 
            
             \\
             \toprule
             RRL~\cite{zeng2017agent}
             & 19.0 & 8.5 & 4.8 & 72.8 & 38.0 & 49.9 & 15.3 & 0.01 & 1.2 & 0.49 & 54.3
             \\
             RRL+smoothing % threshold===0.25
             & 54.7 & 36.3 & 25.7 & 48.6 & 64.6 & 55.4 & 10.1 & 0.03 & 1.5 & 0.39 & 41.8
             \\

             \midrule
             BCP~\cite{li2020make}
             & 7.0 & 3.9 & 3.4  & 48.3 & 26.5 & 34.2 & 22.2 & 0.14 & 9.7 & 0.34 & 39.4
             \\
             BCP+smoothing % threshold===0.18
             & 11.7 & 7.5 & 6.6 & 33.2 & 31.6 & 32.4 & 20.7 & 0.14 & 1.2 & 0.27 & 30.3
             \\
             
              \midrule
            \bottomrule
        \end{tabular}
        
\label{table:consistency}
\end{table*}

\begin{table*}[t!]
    \scriptsize
    \centering
\caption{\textbf{Temporal Consistency} results calculated within 1, 2, and 3 seconds before the critical/collision point. \hank{we can add a new experiments that tests if filter can help planning-awareness evaluation. A simple way is to use random to disturb the consistency.}}       %%%%%% interactive+obstacle+collision
\begin{tabular}
            {@{}l @{\;}@{\;}@{\;} c @{\;}@{\;}@{\;}  c @{\;}@{\;}@{\;}  c @{\;}  c @{\;}  c @{\;}@{\;}@{\;}  c @{\;} c @{\;}@{\;} @{\;} c}
            \toprule
            \multirow{2}{*}{ \begin{tabular}{@{\;}c@{\;}} \end{tabular}} & 
             \multicolumn{3}{@{\;}c}{consistency}  & 

             \multicolumn{2}{@{\;}c@{\;}}{interactive}   & 
             \multicolumn{2}{@{\;}c@{\;}}{obstacle}   & 

             \\
             \cmidrule(lr){2-4}
             \cmidrule(lr){5-6} 
             \cmidrule(lr){7-8}
             &
             \multicolumn{1}{@{\;}c}{1s}&
             \multicolumn{1}{@{\;}c}{2s}&
             \multicolumn{1}{@{\;}c}{3s}& 
              
             \begin{tabular}{c@{\;}@{\;}@{\;}}  IR  \end{tabular} & 
             \begin{tabular}{c@{\;}@{\;}}  CR (\%)  \end{tabular} & 
             \begin{tabular}{c@{\;}@{\;}@{\;}}  IR   \end{tabular} & 
             \begin{tabular}{c@{\;}@{\;}}  CR (\%)  \end{tabular} & 
            
             \\
             \toprule
             RRL~\cite{zeng2017agent}
             & 19.0 & 8.5 & 4.8 & 0.01 & 1.2 & 0.49 & 54.3
             \\
             RRL+smoothing % threshold===0.25
             & 54.7 & 36.3 & 25.7 & 0.03 & 1.5 & 0.39 & 41.8
             \\

             \midrule
             BCP~\cite{li2020make}
             & 7.0 & 3.9 & 3.4  & 0.14 & 9.7 & 0.34 & 39.4
             \\
             BCP+smoothing % threshold===0.18
             & 11.7 & 7.5 & 6.6 & 0.14 & 1.2 & 0.27 & 30.3
             \\
             
              \midrule
            \bottomrule
        \end{tabular}
        
\end{table*}

% --------------
\subsection{Fine-grained Scenario-based Evaluation}
\label{subsec:fine-grained}
\begin{table*}[t!]
    \small
    \centering
    % \resizebox{\textwidth}{!}{
        \begin{tabular}
            {@{}l @{\;}@{\;} c @{\;}@{\;} c @{\;} @{\;}  c @{\;}@{\;}   c @{\;}@{\;}  c @{\;}@{\;}   c @{\;}@{\;}  c @{\;}@{\;}  c @{\;}@{\;}  c @{\;}@{\;}  c @{\;}@{\;} }
            \toprule
            \multirow{1}{*} {\begin{tabular}{@{\;}c@{\;}} Risk Id. Algor. \end{tabular}} & 
             % \multicolumn{1}{c}{Night}  & 
             \multicolumn{1}{c}{Rainy}  & 
             \multicolumn{1}{c}{4-way}   & 
             \multicolumn{1}{c}{3-way} &
             \multicolumn{1}{c}{Straight} &
             \multicolumn{1}{c}{TD low} &
             \multicolumn{1}{c}{TD mid} &
             \multicolumn{1}{c}{TD high} &
             \multicolumn{1}{c}{Average} &
             
            \\
             \toprule
             Random
             & 15.2 & 12.5 & 12.7 & 14.5 & 19.3 & 14.2 & 12.9 & 15.1
             \\
             Range (10m) 
             & 53.4 & 45.4 & 44.7 & 52.0 & 57.1 & 52.4 & 51.8 & 53.6
             \\

            \midrule
             Kalman Filter~\cite{thrun2002probabilistic}
             & 46.7 & 38.7 & 37.8 & 44.0 & 52.9 & 44.7 & 43.7 & 46.7
             \\
             Social-GAN~\cite{social-gan}   
             & 45.7 & 33.5 & 37.0 & 46.6 & 50.4 & 44.1 & 44.1 & 46.0
             \\
             MANTRA~\cite{mantra}
             & 45.0 & 34.3 & 37.2 & 44.9 & 50.0 & 43.5 & 43.2 & 45.4
              \\
             QCNet~\cite{zhou2023query}
             & 46.1 & 35.5 & 35.7 & 46.2 & 51.1 & 44.5 & 44.1 & 46.4
              \\
              
            \midrule
             DSA~\cite{chan2016anticipating} 
             & 46.7 & 38.4 & 46.6 & 39.9 & 46.8 & 46.4 & 47.2 & 46.8
             \\
             RRL~\cite{zeng2017agent}
             & 46.6 & 46.3 & 49.3 & 33.5 & 48.0 & 48.8 & 49.1 & 48.6
             \\
             
             \midrule
             BP~\cite{li2020gcn}
             & 17.7 & 13.9 & 9.4 & 14.4 & 22.1 & 14.2 &  12.6 & 16.6
             \\
             BCP~\cite{li2020make}
             & 33.7 & 20.7 & 24.5 & 37.8 & 36.0 & 32.2 & 31.8 & 33.4
             \\
             \midrule
            \bottomrule
        \end{tabular}
        % }
\caption{Scenario-based performance analysis on weather, road topology, and traffic density. Note that TD denotes traffic density.}     %%%%%% interactive+collision+obstacle+non-interactive
\label{table:attributes}
\end{table*}
